# Supplementary material for: Towards Practical Lipschitz Bandits
Source: arXiv:1901.09277 source file (2021-01-21)
Supplement: Supplementary file 1 [file appendix.tex]

\newpage
% \vspace{10cm} 
\clearpage

\section{Proofs} 

\subsection{Proof of Claim \ref{claim:concentrate}}
\label{app:concentration}

Here we consider the contextual setting outlined in Section \ref{sec:ctucb}. In this setting, the partition is over the joint space of context and arm $\mathcal{Z} \times \mathcal{A}$, and the corresponding auxiliary function in Definition \ref{def:region-selection} and \ref{def:count-mean} are defined over the joint space $\mathcal{Z} \times \mathcal{A}$. 
This setting reduces to a non-contextual setting when the context is set to a fixed value. 

Below, we state and prove a contextual version of Claim \ref{claim:concentrate}. This naturally gives us a proof for Claim \ref{claim:concentrate}. 

\begin{claim}
    \label{claim:concentration-contextual}
    For any context $z$, arm $a$, and time $t$, with probability at most $\frac{1}{t^4}$, we have:
\begin{align}
    &\quad \left| m_{t-1} (z, a) - f(z, a) \right| \\
    &> L \cdot  D(p_{t-1} (z, a)) + C \sqrt{ \frac{ 4 \log t}{ n_{t-1} (z, a)} } \label{eq:claim3}
\end{align} 
for a constant $C$. 
\end{claim}

\begin{proof}
    First of all, when $t = 1$, this is trivially true by Lipschitzness. Now let us consider the case when $t \ge 2$. 
    Let us use $A_1, A_2, \cdots, A_t$ to denote the random variables of arms selected up to time $t$, $Z_1, Z_2, \cdots, Z_t$ to denote the random context up to time $t$ and $Y_1, Y_2, \cdots, Y_t$ to denote random variables of rewards received up to time $t$. 
    Then the random variables $ \left\{ \sum_{t=1}^T \left( f (Z_t, A_t) - Y_t \right) \right\} $ is a martingale sequence.
    % with respect to the filtration $\sigma ( A_1, Y_1, \cdots, A_t, Y_t )$. 
    This is easy to verify since the noise is mean zero and independent. In addition, since there is no randomness in the partition formation (given a sequence of observations), for a fixed $a$, we have the times  $\mathbbm{1} [(Z_t, A_i) \in p_{t-1} (z, a) ] $ ($i \le t$) is measureable with respect to $\sigma (Z_1, A_1, Y_1, \cdots, Z_t, A_t, Y_t)$. Therefore, the sequence $ \left\{ \sum_{i=1}^t \left( f(Z_i, A_i) - Y_i \right) \mathbbm{1} [ (Z_i, A_i) \in p_{t-1} (z, a) ] \right\}_{t = 1}^T $ is a skipped martingale. Since skipped martingale is also a martingale (stopped martingale is also a martingale), we apply the  Azuma-Hoeffding inequality (with sub-Gaussian tails) \citep{shamir2011variant}. For simplicity, we write 
    \begin{align}
        B_t (z,a) &:= C   \sqrt{ \frac{ 4 \log t}{ n_{t-1} (z, a) } } + L\cdot D(p_{t-1} (z, a)). \\
        \mathcal{E}_t^i (z,a) &:=   (Z_i, A_i) \in p_{t-1} (z, a) 
    \end{align}
    Combining this with Lipschitzness, we get there is a constant $C$ (depends on the a.s. bound of the reward, as a result of Hoeffding inequality), such that 
    \begin{align}
        &\quad \mathbb{P} \left\{ \left| m_{t-1} (z, a) - f (z, a) \right| > B_t (z,a) \right\} \nonumber \\ 
        &\le \mathbb{P} \left\{ \left| \frac{ 1}{ n_{t-1} (z, a) }
        \sum_{i=1}^{t-1} \left( f(Z_i, A_i) - Y_i \right) \mathbbm{1} [ \mathcal{E}_t^i (z,a) ] \right| \right. \nonumber \\
        &\quad \left.+ \left| f(z, a) - \frac{ 1 }{ n_{t-1} (z, a ) }  
        \sum_{i=1}^{t-1}  f(Z_i, A_i)  \mathbbm{1} [ \mathcal{E}_t^i (z,a) ] \right| \right. \nonumber \\
        &\quad > \left. C  \sqrt{ \frac{ 4 \log t}{ n_{t-1} (z, a) } } + L\cdot D(p_{t-1} (z, a)) \right\} \label{eq:lipschitz-concentration} \\
        &\le \frac{1}{t^4}, \nonumber 
    \end{align}
    where (\ref{eq:lipschitz-concentration}) uses both the Lipschitzness and the Azuma-Hoeffding's inequality. 
\end{proof}

\subsection{Proof of Claim \ref{claim:single-step-regret}}
\label{app:single-step-regret}

We prove a contextual version of Claim \ref{claim:single-step-regret}, which is first restated Below. Same as in Appendix \ref{app:concentration}, the setting we are considering is outlined in Section \ref{sec:ctucb}.

\begin{claim}
\label{claim:single-step-regret-contextual}
At any $t$,  
with probability at least $1 - \frac{1}{t^4}$, the single step contextual regret satisfies: 
\begin{align*}
    &\quad f(z_t, a_t^*) - f(z_t, a_t) \\
    &\le 2 L\cdot  D(p_{t-1} (z_t, a_t)) + 2 C \sqrt{ \frac{ 4 \log t}{ n_{t-1} (z_t, a_t)} }
\end{align*}
for a constant $C$. Here $a_t^*$ is the optimal arm for the context $z_t$. 
\end{claim}

\begin{proof}
    By Claim \ref{claim:concentration-contextual}, with probability at least $1 - \frac{1}{t^4}$, the following ((\ref{eq:eq-dummy1}) and (\ref{eq:eq-dummy2})) hold simultaneously, 
    \begin{align}
        &\quad m_{t-1} (z_t, a_t) + C \sqrt{ \frac{ 4 \log t }{ n_{t-1} (z_t, a_t) } } + L\cdot D(p_{t-1} (z_t, a_t)) \nonumber  \\
        &\ge m_{t-1} (z_t, a_t^*) + \sqrt{ \frac{ 4 \log t }{ n_{t-1} (z_t, a_t^*) } } + L\cdot D(p_{t-1} (z_t, a_t^*)) \nonumber  \\
        &\ge f(z_t, a_t^*)  \label{eq:eq-dummy1}
    \end{align}
    \begin{align}
        f(z_t, a_t) &\ge m_{t-1} (z_t, a_t) - C \sqrt{ \frac{ 4 \log t }{ n_{t-1} (z_t, a_t) } } \\
        &\quad - L\cdot D(p_{t-1} (z_t, a_t)) . \label{eq:eq-dummy2}
    \end{align}
    This is true since we first take a one-sided version of Hoeffding-type tail bound in (\ref{eq:claim3}), and then take a union bound over the two points $ (z_t,a_t) $ and $ (z_t,a_t^*) $. This first halves the probability bound and then doubles it. Then we take the complementary event to get (\ref{eq:eq-dummy1}) and (\ref{eq:eq-dummy2}) simultaneously hold with probability at least $1 - \frac{1}{t^4}$. We then take another union bound over time $t$, as discussed in the main text. Note that throughout the proof, we do not need to take union bounds over all arms or all regions in the partition. 
    
    Equation \ref{eq:eq-dummy1} holds by algorithm definition. Otherwise we will not select $a_t$ at time $t$. 
    Combine (\ref{eq:eq-dummy1}) and (\ref{eq:eq-dummy2}), and we get 
    \begin{align*}
        &\quad f (z_t, a_t^*) - f(z_t, a_t) \\
        &= f (z_t, a_t^*) - m_{t-1} (z_t, a_t) \\
        &\quad + m_{t-1} (z_t, a_t) - f(z_t, a_t) \\
        &\le 2 C \sqrt{ \frac{ 4 \log t}{n_{t-1} (z_t, a_t)} }  + 2 L\cdot D(p_{t-1} (z_t, a_t)). 
    \end{align*} 
\end{proof}

This proves Claim \ref{claim:single-step-regret} by setting all $z_t$ to a fixed value. 

\subsection{Proof of Proposition \ref{prop}}
\label{app:proof-prop}
\begin{proof} 
For any $x_1, \dots, x_n$ in where the kernel $k_T (\cdot, \cdot)$ is defined, the Gram matrix $ K = \begin{bmatrix}  k_T (x_i, x_j) \end{bmatrix}_{n \times n} $ can be written into block diagonal form where diagonal blocks are all-one matrices and off-diagonal blocks are all zeros with proper permutations of rows and columns. Thus without loss of generality, for any vector $\bm{v} = [v_1, v_2, \dots, v_n] \in \mathbb{R}^n$, $\bm{v}^\top K \bm{v} = \sum_{b = 1}^B \left( \sum_{j:i_j \text{ in block }b } v_{i_j} \right)^2 \ge 0$ where the first summation is taken over all diagonal blocks and $B$ is the total number of diagonal blocks in the Gram matrix.
\end{proof}

% \subsection{Proof of Lemma \ref{lem:point-scattering} (Point Scattering Inequalities)} \label{app:point-scattering} 

% The pr

\subsection{Proof of (\ref{eq:point-scattering-1})} 
\label{app:point-scattering-1}

Consider the partition $ \mathcal{P}_T $ at time $T$. We label the regions of the partitions by $j = 1,2, \cdots, |\mathcal{P}_T|$. Let $t_{j,i}$ be the time when the $i$-th point in the $j$-th region in $\mathcal{P}_T$ being selected. Let $b_j$ be the number of points in region $j$. Since the partitions are nested, we have $1 + n_{t_{j,i} - 1}^0 (x_{t_{j,i}}) \ge i$ for all $i,j$. We have, for $T \ge 1$, 

\begin{align}
    \sum_{t=1}^T\frac{1}{1 + n_{t-1}^0 (x_t)} &= \sum_{j=1}^{|\mathcal{P}_T|}\sum_{i=1}^{b_j} \frac{1}{1 + n_{t_{j,i} - 1}^0 (x_{t_{j,i}}^0 )} \nonumber \\
    &\le \sum_{j=1}^{|\mathcal{P}_T|}\sum_{i=1}^{b_j} \frac{1}{i} \label{eq:ineq} \\
    &\le \sum_{j=1}^{|\mathcal{P}_T|} \left( 1 + \log b_j \right) \nonumber \\
    &= |\mathcal{P}_T| + \sum_{j=1}^{|\mathcal{P}_T|}  \log b_j \nonumber \\ 
    &= |\mathcal{P}_T| + \log  \prod_{j=1}^{|\mathcal{P}_T|} b_j \nonumber \\
    &\le |\mathcal{P}_T| + |\mathcal{P}_T| \log  \frac{T}{|\mathcal{P}_T|}. \label{eq:am-gm},
\end{align}
where (\ref{eq:ineq}) uses $1 + n_{t_{j,i} - 1}^0 (x_{t_{j,i}}) \ge i$ and (\ref{eq:am-gm}) uses AM-GM inequality and that $\sum_{j=1}^{|\mathcal{P}_T|} b_j = T$. 

\subsection{Proof of (\ref{eq:point-scattering-alpha})}
\label{app:point-scattering-alpha}

The idea is similar to that of (\ref{eq:point-scattering-1}). The key observation is stated in the first paragraph in Appendix \ref{app:point-scattering-1}. For $0< \alpha < 1$, 
\begin{align}
    \sum_{t=1}^T \left( \frac{1}{1 + n_{t-1}^0 (x_t)} \right)^{\alpha} &=  \sum_{j=1}^{|\mathcal{P}_T|}\sum_{i=1}^{b_j} \left( \frac{1}{1 + n_{t_{j,i}}^0 (x_{t_{j,i}}^0 )} \right)^\alpha \nonumber \\
    &\le \sum_{j=1}^{|\mathcal{P}_T|}\sum_{i=1}^{b_j} \frac{1}{i^\alpha} \nonumber \\
    &\le \sum_{j=1}^{|\mathcal{P}_T|} \frac{1}{1-\alpha} b_j^{1 - \alpha} \nonumber \\
    &\le \frac{1}{1 - \alpha} |\mathcal{P}_T|^\alpha T^{1 - \alpha} \label{eq:holder},
\end{align}

where (\ref{eq:holder}) is due to the H\"older's inequality and that $\sum_{j=1}^{|\mathcal{P}_T|} b_j = T$.

\subsection{Gap independent bound for UCB1}
\label{app:ucb1}

In the classic UCB1 algorithm, there are $K$ arms with stochastic rewards supported on $[0,1]$. The UCB1 runs by using (\ref{eq:ucb1}). Following our notations, we use $f$ for the expected reward function. Also, in our language, we consider the partition at any time $t$ to be just the set of $K$ arms. In other words, each of the $K$ arms is always itself a region in the partition. For this algorithm, we have, as a direct consequence of the the Hoeffding's inequality,

\begin{align}
    \left| m_{t-1} (a) - f(a) \right| \le  \sqrt{ \frac{ 2 \log T}{ n_{t-1} (a)} } \label{eq:ucb1-concentration}
\end{align} 
with probability at least $1 - \frac{1}{T^2}$. 
Then, from the algorithm definition, we know, at any time $t$, 

\begin{align}
     m_{t-1} (a_t) + \sqrt{ \frac{ 2 \log T}{ n_{t-1} (a_t)} } \ge m_{t-1} (a^*) + \sqrt{ \frac{ 2 \log T}{ n_{t-1} (a^*)} }  . 
\end{align} 

Otherwise, $a_t$ will not be selected at time $t$. With probability at least $1 - \frac{1}{T^2}$, following two inequalities (\ref{eq:eq-dummy5}) and (\ref{eq:eq-dummy6}) hold simultaneously (we first use one-sided Hoeffding inequality, then take a union bound), 
\begin{align}
     m_{t-1} (a_t) + \sqrt{ \frac{ 2 \log T }{ n_{t-1} (a_t)} } &\ge f(a_t)  \label{eq:eq-dummy5}, \\
     m_{t-1} (a^*) - \sqrt{ \frac{ 2 \log T }{ n_{t-1} (a^*)} } &\le f(a^*)
     \label{eq:eq-dummy6}. 
\end{align} 

Combining (\ref{eq:eq-dummy5}) and (\ref{eq:eq-dummy6}), we get 
\begin{align*}
    f(a^*) - f(a_t) \le 2 \sqrt{ \frac{ 2 \log T }{ n_{t-1} (a^*)} }
\end{align*}
as analog to (\ref{eq:single-step-regret}). Now, we can apply the point scattering inequality and get, with probability at least $1 - \frac{1}{T^2}$,

\begin{align}
    &\quad \sum_{t=1}^T \left[ f (a^*) - f(a_t) \right] \\
    &\le \sum_{t=1}^T 2 \sqrt{ \frac{ 2 \log T }{ n_{t-1} (a_t)} } \nonumber \\
    &\le \sqrt{2 \log T} \sqrt{T}   \sqrt{ \sum_{t=1}^T \frac{ 1 }{ n_{t-1} (a_t)} } \label{eq:ucb1-cauchy}   \\
    &\le \sqrt{2 \log T} \sqrt{T} \sqrt{ e | \mathcal{P}_T |  \log \left( 1 + (e - 1) \frac{T }{  | \mathcal{P}_T |  } \right) }  \label{eq:ucb1-point-scattering} \\
    &= \tilde{ \mathcal{O} } \left( \sqrt{KT} \right)
\end{align}
where (\ref{eq:ucb1-cauchy}) uses Cauchy-Schwarz inequality, and (\ref{eq:ucb1-point-scattering}) uses the point scattering inequality (\ref{eq:point-scattering-gp}) and that $|\mathcal{P}_T| = K$. 

\subsection{Proof of Theorem \ref{thm:uniformmesh} and \ref{thm:uniformmeshcontextual} }
\label{app:uniformmesh}

In this section, we provide a proof for Theorem \ref{thm:uniformmesh}. Following the idea of extending Claim \ref{claim:concentrate} to Claim \ref{claim:concentration-contextual} and Claim \ref{claim:single-step-regret} to Claim \ref{claim:single-step-regret-contextual}, the argument generalizes to prove Theorem \ref{thm:uniformmeshcontextual}. 

\begin{proof}
    Let us say at an arbitrary fixed time $t$, we have refined our partitions for $h$ times. Each time we refine our partition, the original cardinality of partitions is multiplied by $2^d$. Recall that during each partition time, we half the diameter (edge-length) of hypercubes. Then after $h$ times of refining, we have all the cubes with diameter $\left(\frac{1}{2} \right)^h$. Since we make changes to the partition only when the region diameters are larger than $t^{- \frac{1}{d+2}}$, we have at time $t$, 
\begin{equation}
    \frac{1}{2^{h-1}} \ge t^{-\frac{1}{d+2}}.
\end{equation}
Otherwise, we will not make $h$ refinement to the partition. 
This implies $2^{h-1} \le t^{\frac{1}{d+2}}$. Since after each partition, each hypercube is splitted into $2^d$ hypercubes, then $|\mathcal{P}_t(a)| = (2^d)^h$, which means $|\mathcal{P}_t(a)| \le 2 t^{\frac{d}{d+2}}$. %The dimension dependent coefficient get cancelled out by $\sqrt{d}$ in our legal partition definition. 

Since this partition formation rule satisfies requirement 1-4 listed in Theorem \ref{thm:regret-bound}, Claims \ref{claim:concentrate} and \ref{claim:single-step-regret} hold. Since $\sum_{t=1}^T \left( f (a^*) - f(a_t) \right) = \sum_{t=1}^{\left\lfloor \sqrt{T} \right\rfloor} \left( f (a^*) - f(a_t) \right) + \sum_{\left\lfloor \sqrt{T} \right\rfloor + 1}^T \left( f (a^*) - f(a_t) \right)$, and from Claim \ref{claim:concentrate} we know with probability at least $1 - \frac{2}{3\left\lfloor \sqrt{T} \right\rfloor ^ 3} $, $f (a^*) - f(a_t) \le \left[ C \sqrt{ \frac{ 4 \log t}{n_{t-1} (a_t)} }  + L\cdot D(p_{t-1} (a_t))  \right] $ hold simultaneously for all $t = \left\lfloor \sqrt{T} \right\rfloor + 1, \cdots, T$. This is a result of taking a union bound at $a_t$ and at $a^*$, and then over $t = \left\lfloor \sqrt{T} \right\rfloor + 1, \cdots, T$. 

Let $E$ be the event 
\begin{align}
    &\left\{ f (a^*) - f(a_t) \le B_t \text{ for all } t = \left\lfloor \sqrt{T} \right\rfloor + 1, \cdots, T \right\}. \\
    &B_t := \left[ C \sqrt{ \frac{ 4 \log t}{n_{t-1} (a_t)} }  + L\cdot D(p_{t-1} (a_t))  \right]
\end{align}

By law of total expectation, we get 

\begin{align}
    &\mathbb{E} R_T = \mathbb{E} \left[ R_T | E \right] \mathbb{P} (E) + \mathbb{E} \left[ R_T | \bar{E} \right] \left( 1 - \mathbb{P} (E) \right) \label{eq:total-exp} \\
    % &\le \mathbb{E} \left[ R_T | E \right] + \mathbb{E} \left[ R_T | \bar{E} \right] \left( 1 - \mathbb{P} (E) \right) \\
    &\le  \sqrt{T}  +  \sum_{t=\left\lfloor \sqrt{T} \right\rfloor }^T \left[ C \sqrt{ \frac{ 4 \log t}{n_{t-1} (a_t)} }  + L\cdot D(p_{t-1} (a_t))  \right] \label{eq:split-sum} \\
    &\quad+ T \frac{1}{ 3 T^{\frac{3}{2}} }  \label{eq:fail-event} \\ 
    &\le 
    \sqrt{T} + C \sqrt{ T \log T} 
    \sqrt{ \sum_{t= 1 }^T  
    \frac{ 1 }{n_{t-1}(a_t)} } \nonumber \\
    &\quad+ L \sum_{t=1}^T (t-1)^{- \frac{1}{d+2}}  + T \frac{1}{3T^{\frac{3}{2}}} 
    \label{eq:eq-dummy3} \\
    &\le 
    \sqrt{T} \\
    &\quad + C \sqrt{ T \log T } 
    \sqrt{ e | \mathcal{P}_T |  \log \left( 1 + (e - 1) \frac{T }{  | \mathcal{P}_T |  } \right) } \\
    &\quad+ L \sum_{t=1}^T  (t-1)^{- \frac{1}{d+2}} +  \frac{T}{3T^{\frac{3}{2}}}  
     \\
    &\le \tilde{\mathcal{O}} \left( T^{\frac{d+1}{d+2}} \right) \label{eq:eq-dummy4} ,
\end{align}
where (\ref{eq:total-exp}) uses the law of total expectation, (\ref{eq:split-sum}) splits the sum into first $\left\lfloor \sqrt{T} \right\rfloor$ terms and the rest $T - \left\lfloor \sqrt{T} \right\rfloor$ terms, 
and (\ref{eq:fail-event}) corresponds to the failure event term "$ \mathbb{E} \left[ R_T | \bar{E} \right] \left( 1 - \mathbb{P} (E) \right) $" (after splitting sum). 
In (\ref{eq:eq-dummy3}), we use the Cauchy-Schwarz inequality and that the the algorithm ensures $D(p_{t-1} ) \le D(p_{t-1} (a)) \le t^{-\frac{1}{d+2}}$. In (\ref{eq:eq-dummy4}) we use the Point Scattering inequality (\ref{eq:point-scattering-gp}). 

\end{proof} 

Then, note that in our simplified version, we assume the reward is properly scaled so that $C = 1$, and the term $D(p_{t-1} (a))$ takes the same value for all $ a \in \mathcal{A} $ and all $t = 1, 2, \cdots, T$ for the \texttt{UniformMesh} algorithm. This recovers the form of Upper Confidence Bound in Algorithm \ref{alg:uniformmesh}.

\section{Tree Fitting Rule in Experiments}
\label{app:tree-fitting}

One nice property of Algorithm \ref{alg:tucb} is that it only imposes loose rules on the partition formation. Therefore we can use a greedy criterion for constructing regression trees to construct the partition. Leaves in a regression tree form a partition of the space. At the same time, a regression tree is designed to fit the underlying function. This property tends to result in an adaptive partition where the underlying function values within each region are relatively close to each other. For this paper, we use the \textit{Mean Absolute Error} ($MAE$) reduction criterion  \citep{breiman1984classification} to adaptively construct a regression tree. More specifically, 
%the regression tree that we use has only one input parameter: minimal $MSE$ reduction allowed $\mu$; and 
%the regression tree recursively splits nodes based on maximal reduction in $MSE$ until the reduction in $MSE$ is always greater than $\mu$. 

a node $\bm{N}$ containing data samples $ \{ (a_1, y(a_1)), (a_2, y(a_2) ), \dots, (a_n, y(a_n)) \}$ is split along a feature (can be randomly selected for scalability) into $\bm{N}_1$ and $\bm{N}_2$ (where $\bm{N}_1 \cup \bm{N}_2 = \bm{N}$ and $\bm{N}_1 \cap \bm{N}_2 = \phi$) such that the following reduction in MAE is maximized:
\begin{align}
MAE(\bm{N}) - \left( \frac{ | \bm{N}_1 | }{| \bm{N} |} MAE(\bm{N}_1) + \frac{|\bm{N}_2|}{|\bm{N}|} MAE(\bm{N}_2) \right) \label{eq:tree-criterion}
\end{align}
where $MAE(\bm{N}) = \frac{1}{|\bm{N}|} \sum_{a_i \in \bm{N}} \left| y(a_i) - \hat{y}(\bm{N}) \right|$ and $\hat{y} ( \bm{N} ) = \frac{1}{|\bm{N}|} \sum_{a_i \in \bm{N}} y(a_i) $. %is the \textit{mean square error} of node $\bm{N}$. 
%\begin{align}
%\frac{1}{ 2 \left| \bm{N} \right| } \sum_{ x_i, x_j \in \bm{N} } \left( y( x_i ), y( x_j ) \right)^2 - \left( \frac{\left| \bm{N}_1 \right|}{\left| \bm{N} \right|} \frac{1}{ 2 \left| \bm{N}_1 \right| } \sum_{ x_i, x_j \in \bm{N}_1 } \left( y( x_i ), y( x_j ) \right)^2 + \frac{\left| \bm{N}_2 \right|}{\left| \bm{N} \right|} \frac{1}{ 2 \left| \bm{N}_2 \right| } \sum_{ x_i, x_j \in \bm{N}_2 } \left( y( x_i ), y( x_j ) \right)^2 \right). \label{eq:tree-criterion}
%\end{align} 
The nodes are recursively split until the maximal possible reduction in $MAE$ is smaller than $\eta$. The leaves are then used to form a partition. Each region is again associated with a corrected mean and corrected count. Using regression trees, we develop the TreeUCB algorithm  (TUCB), and the Contextual TreeUCB algorithm (CTUCB), as summarized in Algorithms \ref{alg:tucb} and \ref{alg:ctucb}.
% Although tree implementation may result in partitions that are not legal, the empirical results show that in practice the heuristic developed based on the regression tree implementation outperforms most state-of-the-art in tuning neural networks as we will see in Section \ref{sec:tune-nn}. 
The code is provided in the supplementary materials, and can also be implemented via the \texttt{scikit-learn} package \citep{scikit-learn}. 

% \subsection{Analysis of Contextual TreeUCB (CTUCB)}
% \label{app:ctucb}

% \newpage

\section{Experiments details} 
\label{app:exp}

\subsection{Synthetic function details} 
\label{app:exp-synthetic}

The (negated) Himmelblau function used for synthetic experiment in Figure \ref{fig:synthetic-function} is 
\begin{align*}
    f (x_1, x_2) = - \left[ (x_1^2 + x_2 - 11 )^2 + (x_1 + x_2^2 - 7)^2 \right],  
\end{align*}
where $x_1, x_2 \in [-5,5]. $

The (negated) Goldstein function used for synthetic experiment in Figure \ref{fig:synthetic-function} is 
\begin{align*}
    f (x_1, x_2) &= -  [ 1 + (x_1 + x_2 + 1)^2  \\
     & \times (19 - 14x_1 + 3x_1^2 - 14x_2 + 6x_1 x_2 + 3x_2^2) ] \\ 
    &\quad [ 30 + (2x_1 - 3x_2 )^2  \\
     &\times (18 - 32 x_1 + 12x_1^2 + 48x_2 -36x_1 x_2 + 27x_2^2) ],
\end{align*}
where $x_1, x_2 \in [-2,2]. $

Note that we rescale the domains of the above functions to $[-0.5, 0.5]^2$, and rescale their ranges to within $[0,1]$ in our experiments. 

For the competing algorithms, the coefficients for the exploration term are all 1 (default for Zooming, Contextual Zooming, and HOO's concent). In particular for HOO, we set $v_1 = 0.1, \rho = 0.1$ (see Algorithm 1 in \citep{bubeck2011x} for details about their $v$ and $\rho$ in HOO's setting).  

Figure \ref{fig:synthetic-function-large} is Figure \ref{fig:synthetic-function} plotted in larger scale.

\begin{figure}[ht!]
\centering
\subfloat[Himmelblau for non-contextual task]{\includegraphics[scale = 0.32]{./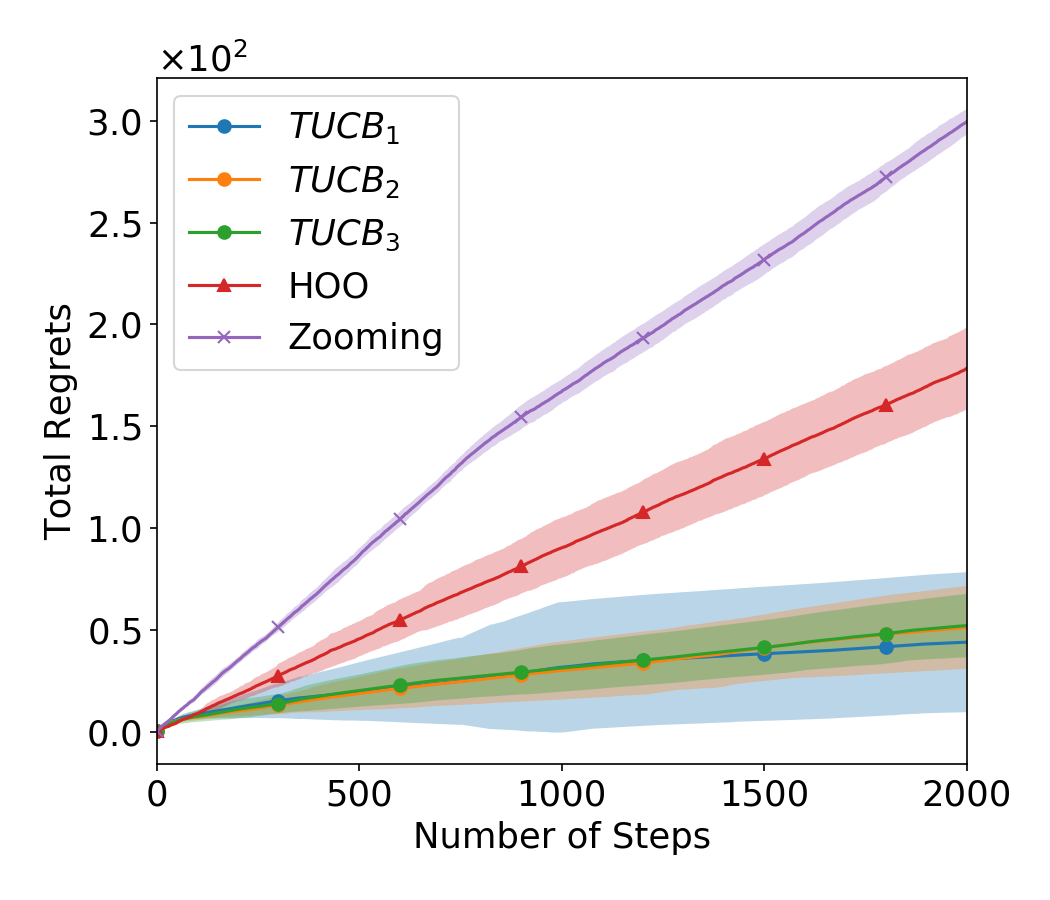} } \\
\subfloat[Goldstein for non-contextual task]{ \includegraphics[scale = 0.32]{./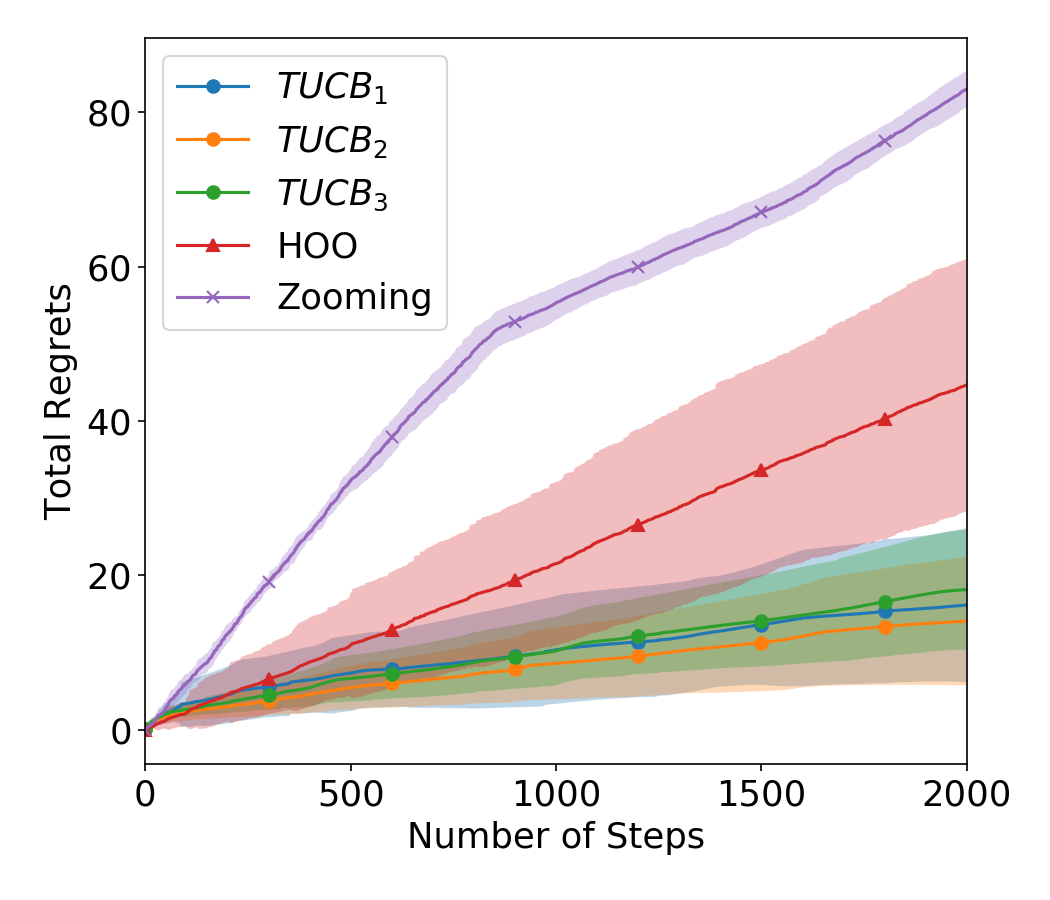} } \\
% \vspace{-1cm}
\subfloat[Himmelblau for contextual task]{\includegraphics[scale = 0.32]{./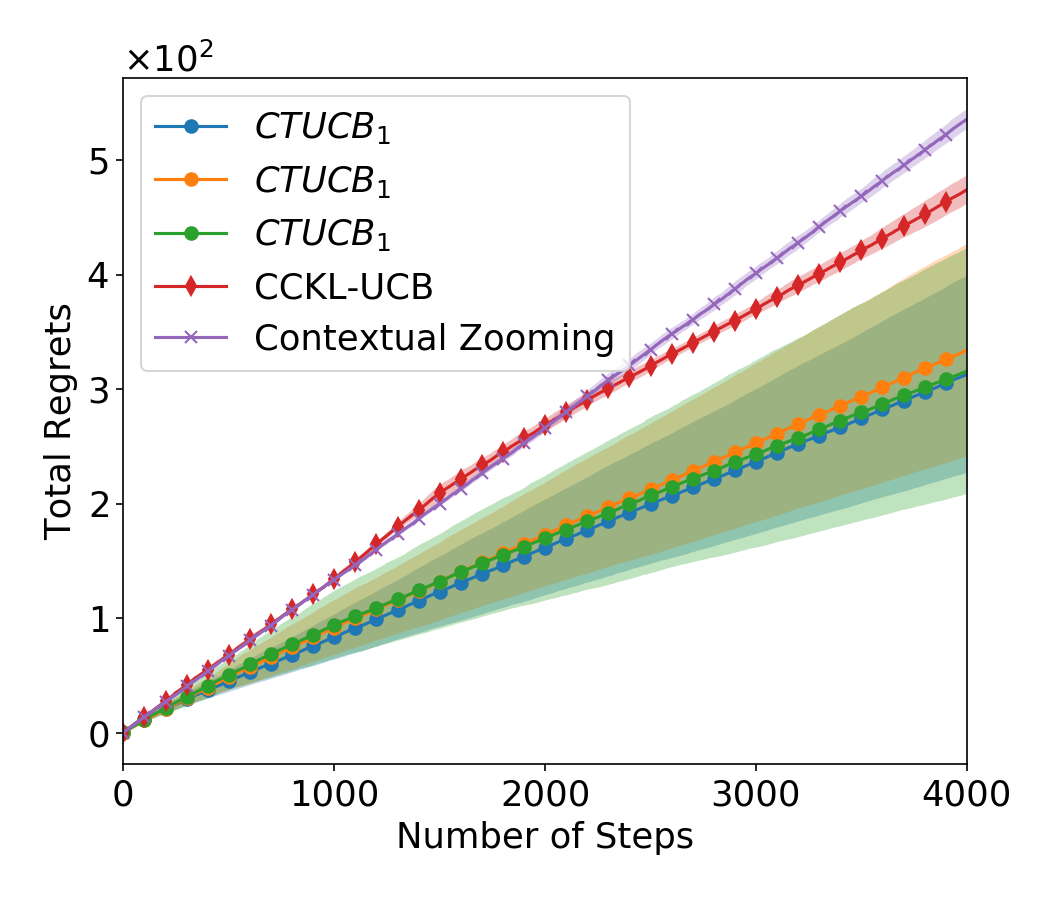} } \\ 
\subfloat[Goldstein for contextual task]{ \includegraphics[scale = 0.32]{./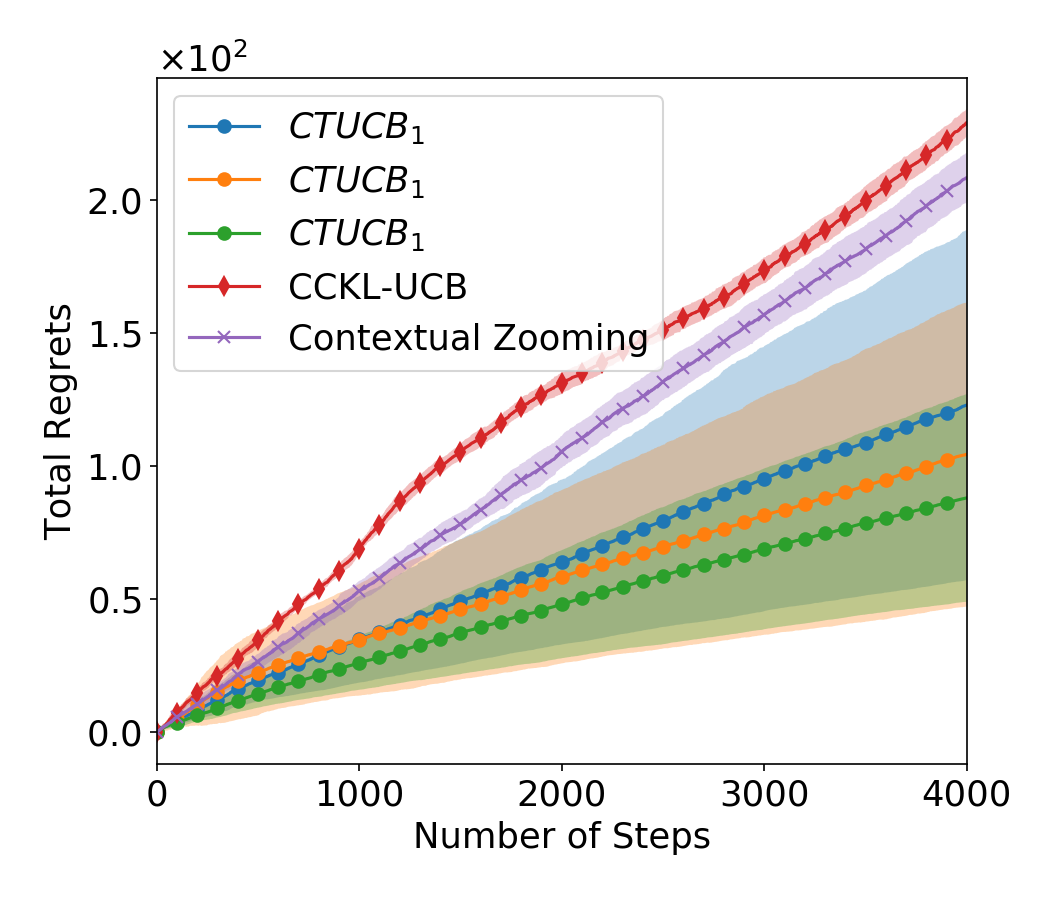} }
% \subfloat[]{\includegraphics[scale = 0.3]{./figures/bandit-compare.png} } \\
% \subfloat[]{ \includegraphics[scale = 0.3]{./figures/bandit-compare-contextual.png} }
% \subfloat[]{\includegraphics[scale = 0.3]{./figures/bandit-compare.png} }
% \subfloat[]{ \includegraphics[scale = 0.3]{./figures/bandit-compare-contextual.png} }\\
%\subfloat[Third.]{ \includegraphics{./figures/fholder1.png}  }%
% \vspace{-0.75cm}
\caption{ Enlarged version of Figure \ref{fig:synthetic-function}.
% \textcolor{red}{This function can easily go in the appendix, and you could just state that it is nonlinear.} 
\label{fig:synthetic-function-large}}
\vspace{-12pt}
\end{figure}

\subsection{The Zooming Rule of Zooming Bandit}

The original Zooming rule in Zooming bandit algorithm, using our notations, can be written as: split a region containing $a$ only when (\ref{eq:zooming-rule}) is violated and no unnecessary splits are made. 
\begin{align}
    D(p_{t-1} (a)) \le \sqrt{\frac{ 8 \log T}{ n_{t-1} (a) } }, \quad a \in [0,1]^d, \label{eq:zooming-rule}
\end{align}
where $T$ is the time horizon. This rule ensures that the range of expected reward within a region (LHS of (\ref{eq:zooming-rule}), due to Lipschitzness) is no larger than Hoeffding-type concentration in the same region (RHS of (\ref{eq:zooming-rule})). For the sake of cleanest representation, the original Zooming rule (\ref{eq:zooming-rule}) assumes both $1$-Lipschitzness (for LHS of (\ref{eq:zooming-rule})) and a proper sub-Gaussian parameter (for RHS of (\ref{eq:zooming-rule})). 

The goal of this rule is to ensure that the Lipschitz term is always dominated by the Hoeffding-type concentration term. When the expected reward is (surjective) onto $[0, K]$ for some $K$, then this rule should be rewritten as 

\begin{align}
    \tilde{K} \cdot D(p_{t-1} (a)) \le \sqrt{ \frac{ 8 \tilde{K}^\prime  \log T}{ n_{t-1} (a) } }, \quad a \in [0,1]^d,
\end{align}
where both $\tilde{K}$ and $\tilde{K}^\prime$ depend on (increase with) $K$. 

When strictly implementing the Zooming bandit algorithm, we should always rescale the rule (\ref{eq:zooming-rule}) when we rescale the reward. 
% If the reward function is simple, we sometimes observe a performance boost if the rewards are rescaled but the rule (\ref{eq:zooming-rule}) is not. This, ironically, is because of an implementation error that should be avoided. 

\subsection{Neural network tuning details}
\label{app:exp-nn}

In this experiment, we use $C = 0.1$, $M = 0.01$ and $\eta = 0.001$ for TUCB. Since the parameter choices are first discretized, we use the following way to compute ``diameter'' of a leaf region in TUCB:
for a leaf region $l$, we count how many points in the discretized parameter space $l$ covers, and use the ratio of this count over total number of discretized grids as the diameter for $l$. All other algorithms use their default setting. 

Figure \ref{fig:tune-nn} in larger scale is in Figure \ref{fig:tune-nn-large} at the end of this document. 

\begin{figure}[ht!]
\centering
\includegraphics[scale = 0.3]{./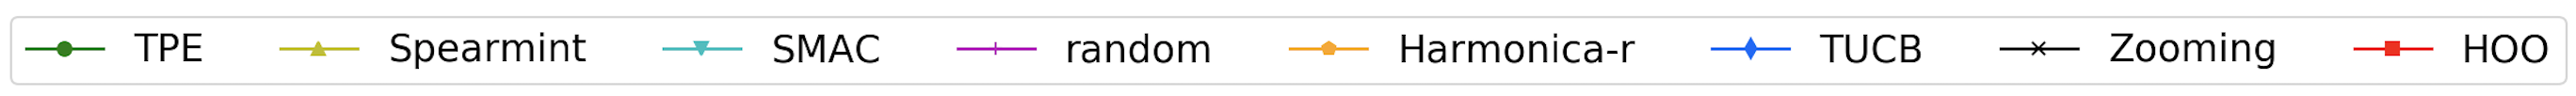} \\
\vspace{-0.4cm}
\subfloat[MLP for MNIST]{\includegraphics[scale = 0.5]{./figures/MNIST_non_contextual.png} \label{fig:tune-nn-mnist-large}} \\
\subfloat[CNN for SVHN]{ \includegraphics[scale = 0.55]{./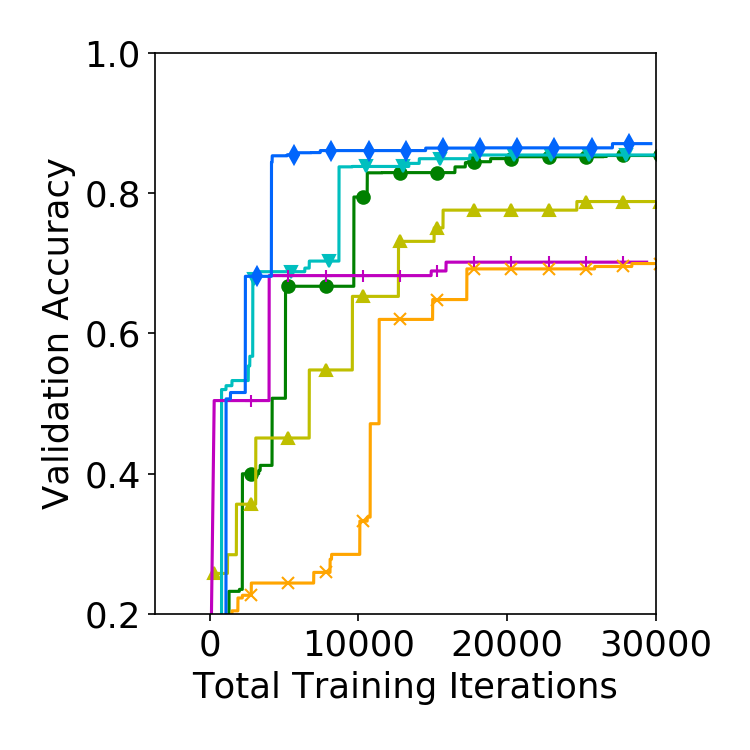} \label{fig:tune-nn-svhn-large}}  \\
\subfloat[CNN for CIFAR-10]{ \includegraphics[scale = 0.5]{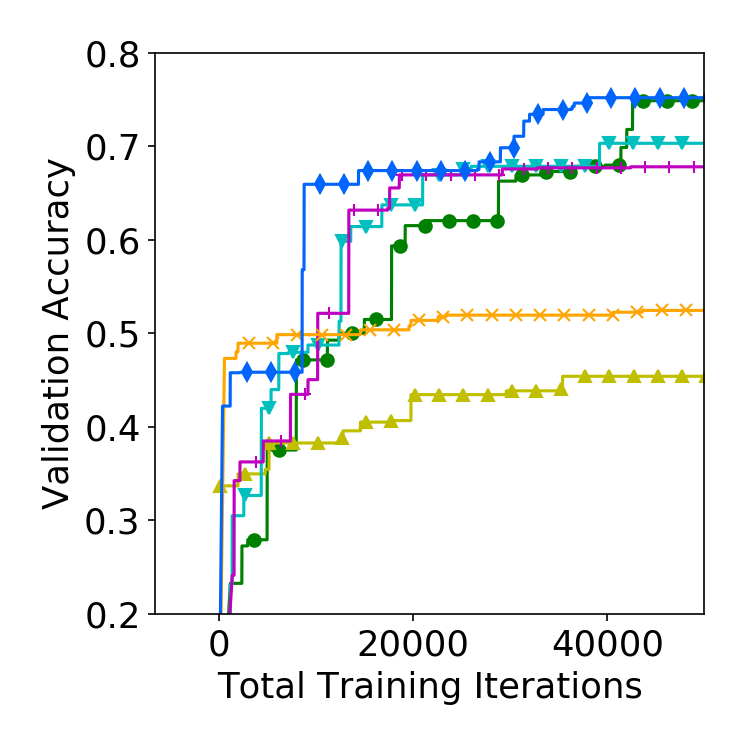}  \label{fig:tune-nn-cifar-large}} 
\caption{Enlarged version of Figure \ref{fig:tune-nn}. \label{fig:tune-nn-large} }
\vspace{-0.6cm}
\end{figure}

\subsubsection{MLP for MNIST}  
\label{sec:mlp-mnist}
% \vspace{-5pt}
The architecture and the hyperparameter space for the simple Multi-Layer Perceptron (MLP) are: in the feed-forward direction, there are the \textit{input layer}, the \textit{fully connected hidden layer with dropout ensemble}, and then the \textit{output layer}. The hyperparameter search space is \textit{number of hidden neurons} (range $[10, 784 ]$), \textit{learning rate}  ($[0.0001, 4 )$), \textit{dropout rate} ($[0.1, 0.9)$), \textit{batch size} ($[10, 500]$), \textit{number of iterations} ($[30, 243]$). 
The settings are for Figure \ref{fig:tune-nn-mnist}. 
% The architecture of this MLP is as follows: 

% As shown in Figure \ref{fig:mlp-mnist}, our methods find good configurations faster than other methods, in both Setting A and Setting B. 

\subsubsection{AlexNet CNN for SVHN}
The architecture of this CNN and the corresponding hyperparameters are summarized in Table \ref{tab:svhn-arch} and \ref{tab:svhn-params}. 
% The results are shown below in Figure \ref{fig:cnn-svhn}. 
%CTUCB saves resources by using information at small iterations to help decisions at larger iterations. The results are summarized in Figure \ref{fig:cnn-svhn}. 
The settings are for Figure \ref{fig:tune-nn-svhn}. 
In this set of experiments, TUCB usually find good configurations at least as fast as other methods. 

\begin{table}[ht!]
\centering
\vspace{1.5cm}
\subfloat[][CNN architecture for SVHN. A value with * means that this parameter is tuned, and the batch-normalization layer uses all Tensorflow's default setting. \label{tab:svhn-arch} ]{
\begin{tabular}{ c c c }
Layer & Hyperparameters & values \\ \hline \hline
\multirow{4}{*}{  Conv1  }  & conv1-kernel-size & *  \\
&  conv1-number-of-channels & 200 \\
&  conv1-stride-size & (1,1) \\
&  conv1-padding & ``same'' \\ \hline
\multirow{3}{*}{  MaxPooling1  }  & pooling1-size & (3,3)  \\
&  pooling1-stride & (1,1) \\
&  pooling1-padding & ``same'' \\ \hline
\multirow{4}{*}{  Conv2  }  & conv2-kernel-size & *  \\
&  conv2-number-of-channels & 200 \\
&  conv2-stride-size & (1,1) \\
&  conv2-padding & ``same'' \\ \hline
\multirow{3}{*}{  MaxPooling2  }  & pooling2-size & (3,3)  \\
&  pooling2-stride & (2,2) \\
&  pooling2-padding & ``same'' \\ \hline
\multirow{4}{*}{  Conv3  }  & conv3-kernel-size & (3,3)  \\
&  conv3-number-of-channels & 200 \\
&  conv3-stride-size & (1,1) \\
&  conv3-padding & ``same'' \\ \hline
\multirow{3}{*}{  AvgPooling3  }  & pooling3-size & (3,3)  \\
&  pooling3-stride & (1,1) \\
&  pooling3-padding & ``same'' \\ \hline
 \multirow{3}{*}{  Dense  }  & batch-normalization & default \\ 
 & number-of-hidden-units & 512 \\ 
 & dropout-rate & 0.5 \\ \hline
\end{tabular}
} 
% \hfill
\vspace{1.5cm}
\subfloat[][Hyperparameter search space. $\beta_1$ and $\beta_2$ are parameters for the AdamOptimizer \citep{kingma2014adam}. The learning rate is discretized in the following way: from 1e-6 to is 1 (including the end points), we log-space the learning rate into 50 points, and from 1.08 to 5 (including the end points) we linear-space the learning rate into 49 points. \label{tab:svhn-params}]{
\begin{tabular}{ c c c }
Hyperparameters & Range  \\ \hline \hline 
conv1-kernel-size & $\{1,2,\cdots,7\}$ \\ \hline 
conv2-kernel-size & $\{1,2,\cdots,7\}$ \\ \hline 
$\beta_1$ & $\{0 , 0.05 ,  \cdots, 1 \}$  \\ \hline 
$\beta_2$ & $\{0 , 0.05 ,  \cdots, 1 |$  \\ \hline 
learning-rate & 1e-6 to 5 \\ \hline 
\makecell{training-iteration } & $\{300,400, \cdots,1500\}$ \\ \hline
\end{tabular}
}
\caption{Settings for the SVHN experiments.}
\end{table}

% \vspace{-2cm}
\subsubsection{AlexNet CNN for CIFAR-10}
% \vspace{-.5cm}
\label{sec:cifar}
% In this section, we tune an AlexNet-type \citep{krizhevsky2012imagenet} CNN \citep{lecun1998gradient} for the CIFAR-10 dataset \citep{krizhevsky2009learning} and compare TUCB and CTUCB with state-of-the-art methods. 
The architecture of this CNN and the corresponding hyperparameters are summarized in Table \ref{tab:cifar-arch} and \ref{tab:cifar-params}. 
The settings are for Figure \ref{fig:tune-nn-cifar}. 

\begin{table}[ht!]
\centering
% \vspace{3cm}
\subfloat[][CNN architecture for CIFAR-10. A value with * means that this parameter is tuned, and the batch-normalization layer uses all Tensorflow's default setting. \label{tab:cifar-arch} ]{
\begin{tabular}{ c c c }
Layer & Hyperparameters & values \\ \hline \hline
\multirow{4}{*}{  Conv1  }  & conv1-kernel-size & *  \\
&  conv1-no.-of-channels & 200 \\
&  conv1-stride-size & (1,1) \\
&  conv1-padding & ``same'' \\ \hline
\multirow{3}{*}{  MaxPooling1  }  & pooling1-size & *  \\
&  pooling1-stride & (1,1) \\
&  pooling1-padding & ``same'' \\ \hline
\multirow{4}{*}{  Conv2  }  & conv2-kernel-size & *  \\
&  conv2-no.-of-channels & 200 \\
&  conv2-stride-size & (1,1) \\
&  conv2-padding & ``same'' \\ \hline
\multirow{3}{*}{  MaxPooling2  }  & pooling2-size & *  \\
&  pooling2-stride & (2,2) \\
&  pooling2-padding & ``same'' \\ \hline
\multirow{4}{*}{  Conv3  }  & conv3-kernel-size & *  \\
&  conv3-no.-of-channels & 200 \\
&  conv3-stride-size & (1,1) \\
&  conv3-padding & ``same'' \\ \hline
\multirow{3}{*}{  AvgPooling3  }  & pooling3-size & *  \\
&  pooling3-stride & (1,1) \\
&  pooling3-padding & ``same'' \\ \hline
 \multirow{3}{*}{  Dense  }  & batch-normalization & default \\ 
 & no.-of-hidden-units & 512 \\ 
 & dropout-rate & 0.5 \\ \hline
\end{tabular}
} \hfill
\subfloat[][Hyperparameter search space. $\beta_1$ and $\beta_2$ are parameters for the Adamoptimizer. The learning rate is discretized in the following way: from 1e-6 to is 1 (including the end points), we log-space the learning rate into 50 points, and from 1.08 to 5 (including the end points) we linear-space the learning rate into 49 points. The learning-rate-reduction parameter is how many times the learning rate is going to be reduced by a factor of 10.
For example, if the total training iteration is 200, the learning-rate is 1e-6, and the  
learning-rate-reduction is 1, then for the first 100 iteration the learning rate is 1e-6, and the for last 100 iterations the learning rate is 1e-7. \label{tab:cifar-params}]{
\begin{tabular}{ c c c }
Hyperparameters & Range  \\ \hline \hline 
conv1-kernel-size & $\{1,2,\cdots,7\}$ \\ \hline  
conv2-kernel-size & $\{1,2,\cdots,7\}$ \\ \hline  
%& $\{1,2,\cdots,7\}$ \\ \hline 
conv3-kernel-size & $\{1,2,3 \}$ \\ \hline 
pooling1-size  & $\{1,2,3\}$ \\ \hline 
pooling2-size & $\{1,2,3\}$ \\ \hline 
pooling3-size & $\{1,2,\cdots, 6 \}$ \\ \hline 
$\beta_1$ \& $\beta_2$ & $\{0 , 0.05 ,  \cdots, 1 \}$  \\ \hline 
learning-rate & 1e-6 to 5 \\ \hline
learning-rate-redeuction & \{1,2,3\} \\ \hline
\makecell{training-iteration } & $\{200,400, \cdots,3000\}$ \\ \hline
\end{tabular}
}
\vspace{0.1cm}
\caption{Settings for CIFAR-10 experiments. 
}
\end{table}

% As shown in Figure \ref{fig:tune-tucb}, our methods find good configurations faster than other methods most of the time.
In particular,  TUCB reaches 70\% accuracy using 30,400 iterations, while other methods on average require 42,800 iterations. 
% in Setting B, TUCB reaches 70\% accuracy using 11,943 iterations, while other methods on average require 71,934 total iterations.

\section{Installation of TUCB}

In our neural network experiments, TUCB is implemented using a modified \texttt{scikit-learn} package. The users need to reinstall \texttt{scikit-learn} using the package provided in the supplement in order to run TUCB (and CTUCB). To install the modified \texttt{scikit-learn} package, the users need to 1) uninstall the original \texttt{scikit-learn} package (for example, using the following command); 
\begin{minted}{bash}
  $ pip uninstall scikit-learn
\end{minted}

2) unzip the ``scikit-learn-modified.zip" file, navigate into the unzipped folder, and run one of the following commands from a Linux terminal (tested on Ubuntu 16.04 and 18.04 with Python 3.6).

\begin{minted}{bash}
  $ python setup.py install 
\end{minted}
The user might need the run the following command as well, if there is a 32-bit versus 64-bit inconsistency between the OS and the package. 
\begin{minted}{bash}
  $ apt-get install gcc-multilib 
\end{minted}
Mac OS and Windows systems should be able to install the package with similar commands, but those systems can have different default compilers. The users may face difficulty in installation. It is highly recommended to use Linux systems. The users could also consult \url{https://scikit-learn.org/stable/developers/advanced_installation.html} for more detailed on build and install \texttt{scikit-learn} from source. Please contact the authors if faced with difficulties.
